# Supplementary material for: Doubly Robust Counterfactual Classification
Source: arXiv:2301.06199 source file (2023-01-15)
Supplement: Supplementary file 1 [file appendix_old.tex]

\section{Additional Technical Results}
The following lemma suggests an efficient method to estimate each unknown component of \eqref{eqn:true-opt-problem}.

\begin{lemma} \label{prop:double-robust}
For some $g: \mathcal{Y} \rightarrow \R$ and $h_w: \mathcal{W} \rightarrow \R$, let $\mu_{g,a}=\E[g(Y) \mid X,S, A=a]$, so $\eta=\{\pi_a, \mu_{g,a}\}$. Also, define our parameter and the corresponding estimator by $\psi_{g,a} = \E[g(Y^a)h_w(W)]$, $\widehat{\psi}_{g,a}=\Pb\{\varphi_a(g(Y);\widehat{\eta})h_w(W)\}$, respectively. If we assume that:
\begin{enumerate}[label={}, leftmargin=*]
	    \item \customlabel{assumption:B1}{(B1)} either 1) $\widehat{\eta}$ are estimated using sample splitting or 2) the function class  $\{\varphi_a(\cdot;\eta): \eta \in (0,1)^2\times \R^2\}$ is Donsker in $\eta$
	    \item \customlabel{assumption:B2}{(B2)}  $\Pb(\widehat{\pi}_a \in [\epsilon, 1-\epsilon]) = 1$ for some $\epsilon > 0$ 
	    \item \customlabel{assumption:B3}{(B3)} $\Vert \widehat{\mu}_{g,a}- \mu_{g,a} \Vert_{2,\Pb} = o_\Pb(1)$,
\end{enumerate}	    
Then we have
\begin{align*}
    \Vert \widehat{\psi}_a - \psi_a \Vert_2 &= O_\Pb\left(\Vert \widehat{\pi}_a - \pi_a \Vert_{2,\Pb} \Vert \widehat{\mu}_{g,a}- \mu_{g,a} \Vert_{2,\Pb} \right).
\end{align*}
If we further assume that
\begin{enumerate}[label={}, leftmargin=*]	    
	    \item \customlabel{assumption:B4}{(B4)}  
	    $   \begin{aligned}[t]
            &\Vert \widehat{\psi}_{g,a} - {\psi}_{g,a} \Vert_{2,\Pb} \Vert \widehat{\mu}_{g,a} - \mu_{g,a} \Vert_{2,\Pb} = o_\Pb(n^{-1/2}), 
            \end{aligned} 
        $
\end{enumerate}
then
\begin{align} \label{eqn:asymptotic-psi}
    \sqrt{n}(\widehat{\psi}_{g,a} - {\psi}_{g,a}) \xrightarrow[]{d} N\left(0,\var\left(\varphi_a(g(Y);\eta)h_w(W)\right)\right),
\end{align}
and the estimator $\widehat{\psi}_{g,a} $ is efficient, meaning no other estimators have smaller asymptotic variance.
\end{lemma}


\section{Proofs}
\textbf{Extra notations.} We let $\mathbb{B}_r(z)$ denote an open ball of radius $r$ centered at $z$, and let $M_l$ and $v_l$ denote the $l$-th row and the $l$-th element in a matrix $M$ and a vector $v$, respectively. We use $(M)_{ij}$ to denote the $(i,j)$-element of the matrix $M$. Further, we let $\Vert M \Vert_F$ denote the Frobenius norm. $\Vert \cdot \Vert_2$ is understood as the spectral norm when it is used with a matrix.

Further, we let $o_{x \rightarrow \alpha}(1)$ denote some function of $x$ that converges to $0$ when $x \rightarrow \alpha$, i.e., a function $\mathsf{h}_{\alpha}(x): \mathcal{X} \rightarrow \mathbb{R}^r$ such that $\underset{x \rightarrow \alpha}{\lim} \bar{\mathsf{h}}_{\alpha}(x)_j = 0$, $\forall j = 1,...,r$ where $r \geq 1$ is appropriately determined by context. This is to distinguish from typical little-o ($o$) asymptotic notation with respect to $n$ in our proofs.


\subsection{Proof of Theorem \ref{thm:convergence-rates}}
\label{appendix:proof-convergence-rates}

We consider a more general case of stochastic nonlinear programming with the deterministic linear constraints; suppose we are concerned with the following true and approximating programs with some finite-dimensional decision variable $x$ in some compact subset $\mathcal{S} \in \R^k$.

\begin{minipage}{.5\textwidth}
\begin{equation}
\label{eqn:true-nlp-linear-constraints}
    \begin{aligned}
        &\underset{x \in \mathcal{S}}{\text{minimize}} \quad f(x) \\
        & \text{subject to} \quad Cx \leq d
    \end{aligned} \tag{$\mathsf{P}$}  
\end{equation} 
\end{minipage}%
\hfill
\begin{minipage}{.5\textwidth}
\begin{equation}
\label{eqn:approx-nlp-linear-constraints}
    \begin{aligned}
        & \underset{x \in \mathcal{S}}{\text{minimize}} \quad \widehat{f}(x) \\
        & \text{subject to} \quad \widehat{C} x \leq \widehat{d}
    \end{aligned} \tag{$\widehat{\mathsf{P}}$}  
\end{equation}
\end{minipage}

We introduce the \textit{active index set} for our inequality constraints.
\begin{definition}[Active set]
For $\bar{x}$ in the feasible set, the active index set $J_0$ is defined by
\[
J_0(\bar{x}) = \{1\leq j \leq m \mid C_j^\top\bar{x} = d_j \}.
\]
\end{definition}

We first give the following useful lemmas.

\begin{lemma} \label{lem:appendix-1}
Let $\widehat{x}$ be an optimal solution of \ref{eqn:approx-nlp-linear-constraints}. Assume that both $f, \widehat{f}$ are twice Frechet-differentiable with respect to $x$.
Then we have 
\begin{align*}
    \dist\left(\widehat{x} , \sol(\text{\ref{eqn:true-nlp-linear-constraints}})\right) &= O_\Pb\left(\Vert \nabla_x\widehat{f}(x^*) - \nabla_xf(x^*) \Vert + \Vert \widehat{C} - C \Vert + \Vert\widehat{d} - d \Vert \right).
\end{align*}
Thus, $\widehat{x}$ is consistent if \ref{eqn:approx-nlp-linear-constraints} is componentwise consistent.
\end{lemma}

\begin{proof}
First note that since \ref{eqn:true-nlp-linear-constraints} and \ref{eqn:approx-nlp-linear-constraints} have feasible sets that consist of only linear inequalities, the KKT optimality conditions hold for the both \citep[][Theorem 5.4]{faigle2013algorithmic}. Let $\gamma$ and $\widehat{\gamma}$ be the dual variables for \ref{eqn:true-nlp-linear-constraints} and \ref{eqn:approx-nlp-linear-constraints}, respectively. Pick $\forall x^* \in \sol(\text{\ref{eqn:true-nlp-linear-constraints}})$. Then from the complementary slackness, for each $j \in \{1,...,m\}$, we have $\gamma_j (C_jx^*-d_j) =0$ and $\widehat{\gamma}_j (C_j\widehat{x}-\widehat{d}_j) =0$, and thus
\begin{align*}
    \gamma_j (C_jx^*-d_j) - \widehat{\gamma}_j (\widehat{C}_j\widehat{x}-\widehat{d}_j) &= (\gamma_j - \widehat{\gamma}_j)(C_jx^*-d_j) + \widehat{\gamma}_j\left\{(C_jx^*-d_j) - (\widehat{C}_j\widehat{x}-\widehat{d}_j)\right\} \\
    &= (\gamma_j - \widehat{\gamma}_j)(C_jx^*-d_j) + \widehat{\gamma}_jC_j(x^* -\widehat{x}) 
    + \widehat{\gamma}_j\left\{ (C_j - \widehat{C}_j)\widehat{x} +\widehat{d}_j - d_j\right\} \\
    & = 0.
\end{align*}
By Cauchy Schwarz inequality, this leads to
\begin{equation} \label{aux-eqn:lemma-1-1}
\begin{cases}
    j \notin J_0(x^*) \, \Rightarrow \, \widehat{\gamma}_j - \gamma_j  = O\left( \Vert \widehat{x}- x^* \Vert + \Vert \widehat{C}_j- C_j \Vert + \vert \widehat{d}_j- d_j \vert \right),
    \\
    j \in J_0(x^*) \, \Rightarrow \, \widehat{\gamma}_j = 0 .
\end{cases}
\end{equation}
Now, from the stationary conditions, by adding and subtracting terms it follows
\begin{align*}
 0 &= \nabla_x\widehat{f}(\widehat{x}) - \nabla_xf(x^*) + \sum_j\left\{ \widehat{\gamma}_j\widehat{C}_j^\top - \gamma_jC_j^\top \right\} \\
 &= \nabla_x\widehat{f}(\widehat{x}) - \nabla_x\widehat{f}(x^*) + \nabla_x\widehat{f}(x^*) - \nabla_xf(x^*) 
 + \sum_j\left\{(\widehat{\gamma}_j-\gamma_j)\widehat{C}_j^\top + \gamma_j(\widehat{C}_j^\top- C_j^\top)\right\} \\
 & = (\widehat{x} - x^*)^\top \nabla^2_{x}\widehat{f}(x^*) + (\widehat{x} - x^*) o_{\widehat{x} \rightarrow x^*}(1) + \nabla_x\widehat{f}(x^*) - \nabla_xf(x^*) \\
 & \quad + \sum_j\left\{(\widehat{\gamma}_j-\gamma_j)\widehat{C}_j^\top + \gamma_j(\widehat{C}_j^\top- C_j^\top)\right\},
\end{align*}
where the last equality follows by Taylor's theorem.

Hence, by applying \eqref{aux-eqn:lemma-1-1} to the last display above, we obtain
\begin{align*}
\Vert \widehat{x}-x^* \Vert\left\{O(1) + o_{\widehat{x} \rightarrow x^*}(1) \right\} & \leq \Vert \nabla_x\widehat{f}(x^*) - \nabla_xf(x^*) \Vert + O\left(\sum_j \vert \widehat{\gamma}_j - \gamma_j  \vert \right) \\
& \Vert \widehat{x}-x^* \Vert\left\{O(1) + o_{\widehat{x} \rightarrow x^*}(1) \right\} +\nabla_x\widehat{f}(x^*) - \nabla_xf(x^*)  + O\left( \sum_j \left\{ \vert \widehat{d}_j - d_j  \vert + \Vert \widehat{C}_j^\top - {C}_j^\top \Vert \right\} \right) \\
& = 0.
\end{align*}

Hence, from the given consistency conditions that $\Vert \nabla_x\widehat{f} - \nabla_xf \Vert = o_\Pb(1)$, $\vert \widehat{d}_j - d_j \vert = o_\Pb(1)$ and $\Vert \widehat{C}_j^\top - {C}_j^\top \Vert = o_\Pb(1)$, we get 
\[
    \Vert \widehat{x} - x^* \Vert = 
\]
which leads to the conclusion $\Vert \widehat{x} - x^* \Vert = o_\Pb(1)$. From $\dist(x^*, \sol(\mathsf{P}(\widehat{x}))) \leq \Vert \widehat{x} - x^* \Vert$, the desired result follows.
\end{proof}

\begin{lemma} \label{lem:appendix-2}
Under the same conditions of Lemma \ref{lem:appendix-1}, if we further assume that $f$ is convex, we have
\begin{align*}
    \dist\left(\widehat{x} , \sol(\text{\ref{eqn:true-nlp-linear-constraints}})\right) = O_\Pb\left( \Vert \nabla_x^2\widehat{f}(x^*) - \nabla_x^2 f(x^*)  \Vert \right).
\end{align*}
\end{lemma}

\begin{proof}
Pick $x^*$, $\widehat{x}$ such that $\Vert \widehat{x} - x^* \Vert = \dist(x^*, \sol(\mathsf{P}(\widehat{\theta})))$. 

By Taylor's theorem
\begin{align*}
    \widehat{f}(\widehat{x}) = \widehat{f}(x^*) + \nabla_x\widehat{f}(x^*)^\top(\widehat{x}-x^*) + \frac{1}{2}(\widehat{x}-x^*)^\top \nabla_x^2\widehat{f}(x^*) (\widehat{x}-x^*) + o_{\widehat{x} \rightarrow x^*}\left(\Vert \widehat{x}-x^* \Vert^2 \right).
    % O\left(\mathsf{h}_{x^*}(\widehat{x}) \Vert  \widehat{x} - x^* \Vert^2\right),
\end{align*}

Since $\widehat{f}(\widehat{x}) - \widehat{f}(x^*) \leq 0$, $\forall x^*, \widehat{x} \in \mathcal{S}$, by adding and subtracting terms from the above equality, we get
\begin{align}\label{eqn:proof-1-disp-1}
     0 
     & \geq \nabla_x\widehat{f}(x^*)^\top(\widehat{x}-x^*) + \frac{1}{2}(\widehat{x}-x^*)^\top \nabla_x^2\widehat{f}(x^*) (\widehat{x}-x^*) + o_{\widehat{x} \rightarrow x^*}\left(\Vert \widehat{x}-x^* \Vert^2 \right) \nonumber \\
     & = \left\{\nabla_x\widehat{f}(x^*) - \nabla_xf(x^*) \right\}^\top(\widehat{x}-x^*) + \nabla_xf(x^*)^\top(\widehat{x}-x^*) \nonumber\\
     & \quad + \frac{1}{2}(\widehat{x}-x^*)^\top \left\{ \nabla_x^2\widehat{f}(x^*) - \nabla_x^2 f(x^*) + \nabla_x^2 f(x^*) \right\} (\widehat{x}-x^*) + o_{\widehat{x} \rightarrow x^*}\left(\Vert \widehat{x}-x^* \Vert^2 \right)  \nonumber  \\
     & = \left\{\nabla_x\widehat{f}(x^*) - \nabla_xf(x^*) \right\}^\top(\widehat{x}-x^*) + \nabla_xf(x^*)^\top(\widehat{x}-x^*) \nonumber \\
     & \quad + \frac{1}{2}(\widehat{x}-x^*)^\top \left\{ \nabla_x^2\widehat{f}(x^*) - \nabla_x^2 f(x^*) \right\} (\widehat{x}-x^*) + \frac{1}{2}(\widehat{x}-x^*)^\top \nabla_x^2 f(x^*) (\widehat{x}-x^*) + o_{\widehat{x} \rightarrow x^*}\left(\Vert \widehat{x}-x^* \Vert^2 \right).
\end{align}

Since we only have linear inequalities in \ref{eqn:true-nlp-linear-constraints} and $\nabla_x^2 f(x^*)$ is positive definite, the quadratic growth condition holds at $x^*$ \citep[][Theorem 2.4]{still2018lectures}. Namely with some $\delta^* >0$ and $\kappa >0$ it holds:
\[
f(\widehat{x}, {\theta})  - f(x^*, {\theta}) \geq \kappa \Vert \widehat{x}-x^* \Vert^2 \quad  \forall \widehat{x} \in \mathbb{B}_{\delta}(x^*).
\]

Hence, again from Taylor's theorem it follows
\begin{align*}
    &\nabla_xf(x^*, {\theta})^\top(\widehat{x}-x^*) + \frac{1}{2}(\widehat{x}-x^*)^\top \nabla_x^2f(x^*, {\theta}) (\widehat{x}-x^*) \\
    &= f(\widehat{x}, {\theta})  - f(x^*, {\theta}) + o_{\widehat{x} \rightarrow x^*}\left(\Vert \widehat{x}-x^* \Vert^2 \right)\\
    & \geq  \kappa \Vert \widehat{x}-x^* \Vert^2 + o_{\widehat{x} \rightarrow x^*}\left(\Vert \widehat{x}-x^* \Vert^2 \right).
\end{align*}

By applying this result to \eqref{eqn:proof-1-disp-1}, we have
\begin{align*}
    0 &\geq \left\{\nabla_x\widehat{f}(x^*) - \nabla_xf(x^*) \right\}^\top(\widehat{x}-x^*) + \frac{1}{2}(\widehat{x}-x^*)^\top \left\{ \nabla_x^2\widehat{f}(x^*) - \nabla_x^2 f(x^*) \right\} (\widehat{x}-x^*) \\
    & \quad + \kappa \Vert \widehat{x}-x^* \Vert^2 + o_{\widehat{x} \rightarrow x^*}\left(\Vert \widehat{x}-x^* \Vert^2 \right).
\end{align*}

By the Cauchy–Schwarz inequality,
\begin{align*}
    \left\{1 + o_{\widehat{x} \rightarrow x^*}(1) \right\}\Vert \widehat{x}-x^* \Vert^2 \lesssim \Vert \widehat{x}-x^* \Vert \left\{  \Vert \nabla_x\widehat{f}(x^*) - \nabla_xf(x^*) \Vert + \Vert \widehat{x}-x^*\Vert \Vert \nabla_x^2\widehat{f}(x^*) - \nabla_x^2 f(x^*) \Vert_F \right\}.
\end{align*}

Given that $\Vert \nabla_x^2\widehat{f}(x^*) - \nabla_x^2 f(x^*) \Vert_F = o_{\Pb}(1)$, the above inequality forces that $\left\Vert \widehat{x}-x^* \right\Vert = O_\Pb \left(\left \Vert \nabla_x\widehat{f}(x^*) - \nabla_xf(x^*) \right\Vert\right)$.
\end{proof}

\begin{proof}
Let $\gamma$ and $\widehat{\gamma}$ be the dual variables for \ref{eqn:true-nlp-linear-constraints} and \ref{eqn:approx-nlp-linear-constraints}, respectively.
We first aim to show that
\begin{align} \label{eqn:appendix-proof2-2}
    \Vert \widehat{\gamma}_j-\gamma_j \Vert = O_\Pb \left( \Vert \widehat{x} - x^* \Vert  + n^{-1/2} \right).
\end{align}

To this end, we note that since \ref{eqn:true-nlp-linear-constraints} and \ref{eqn:approx-nlp-linear-constraints} have feasible sets that consist of only linear inequalities, the KKT optimality conditions hold for the both \citep[][Theorem 5.4]{faigle2013algorithmic}.  From the stationary conditions, by adding and subtracting terms it follows
\begin{align*}
 0 &= \nabla_x\widehat{f}(\widehat{x}) - \nabla_xf(x^*) + \sum_j\left\{ \widehat{\gamma}_j\widehat{C}_j^\top - \gamma_jC_j^\top \right\} \\
 &= \nabla_x\widehat{f}(\widehat{x}) - \nabla_x\widehat{f}(x^*) + \nabla_x\widehat{f}(x^*) - \nabla_xf(x^*) 
 + \sum_j\left\{(\widehat{\gamma}_j-\gamma_j){C}_j^\top + \widehat{\gamma}_j(\widehat{C}_j^\top- C_j^\top)\right\} \\
 & = (\widehat{x} - x^*)^\top \nabla^2_{x}\widehat{f}(x^*) + (\widehat{x} - x^*) o_{\widehat{x} \rightarrow x^*}(1) + \nabla_x\widehat{f}(x^*) - \nabla_xf(x^*) \\
 & \quad + \sum_j\left\{(\widehat{\gamma}_j-\gamma_j){C}_j^\top + \widehat{\gamma}_j(\widehat{C}_j^\top- C_j^\top)\right\},
\end{align*}
where the last equality follows by Taylor's theorem. Since we have assumed non-zero rows in $C$, by the Cauchy–Schwarz and triangle inequalities we obtain
\begin{align*}
    \Vert \widehat{\gamma}_j-\gamma_j \Vert &\lesssim \Vert \widehat{x} - x^* \Vert  + \Vert \nabla_x\widehat{f}(x^*) - \nabla_xf(x^*) \Vert  + \Vert \widehat{C} - C \Vert \\
    & \leq \Vert \widehat{x} - x^* \Vert  + \Vert \nabla_x\widehat{f}(x^*) - \nabla_xf(x^*) \Vert_F  + \Vert \widehat{C} - C \Vert_F.
\end{align*}
Note that under the nonparametric condition \ref{}, we get the desired result \eqref{eqn:appendix-proof2-2}. 

Next, consider the following perturbed parametrized program \ref{eqn:true-parametrized-nlp-linear-constraints}:
\begin{equation}
\label{eqn:true-parametrized-nlp-linear-constraints}
    \begin{aligned}
        &\underset{x \in \mathcal{S}}{\text{minimize}} \quad f(x) + x^\top\xi_1 \\
        & \text{subject to} \quad Cx - d - \xi_2 \leq 0,
    \end{aligned} \tag{$\mathsf{P}_\xi$}  
\end{equation} 
for a parameter $\xi = (\xi_1, \xi_2) \in \R^k \times \R^m$. Let $\bar{x}(\xi)$ denote the solution of the program \ref{eqn:true-parametrized-nlp-linear-constraints}. Clearly, we get $\bar{x}(0) = x^*$.

We have already shown that $\widehat{x} \xrightarrow[]{p} x^*$ in Theorem \ref{thm:convergence-rates}. Hence by \citet[][Theorem 3.1]{shapiro1993asymptotic}, we get
\begin{align*}
    \widehat{x} = \bar{x}(\zeta) + o_\Pb(n^{-1/2})
\end{align*}
where 
\begin{align*}
    \zeta = \begin{bmatrix}
    \nabla_x\widehat{f}(x^*) - \nabla_xf(x^*) - \sum_j\gamma_j\left\{ \widehat{C}_j^\top - C_j^\top \right\} \\
    (\widehat{C} - C)x^*
    \end{bmatrix} \equiv \begin{bmatrix}
    \zeta_1 \\
    \zeta_2
    \end{bmatrix}.
\end{align*}
We are particularly interested in $\bar{x}(\zeta)$. If $\bar{x}(\xi)$ is Frechet differentiable at $\xi=0$, we have
\begin{align*}
    \bar{x}(\xi) - x^* = D_0\bar{x}(\xi) + o(\Vert\xi\Vert),
\end{align*}
for some mapping $D_0\bar{x}: \R^k \rightarrow \R^k$. Under the given conditions this leads to
\begin{align*}
    n^{1/2}\left(\widehat{x} - x^* \right) = D_0\bar{x}(n^{1/2}\zeta) + o_\Pb(1).
\end{align*}

By Lemma \ref{lem:} and the delta theorem, it follows that
\begin{align*}
    n^{1/2}\zeta \xrightarrow{d} \begin{bmatrix}
    \nabla_x\widehat{f}(x^*) - \nabla_xf(x^*) - \sum_j\gamma_j\left\{ \widehat{C}_j^\top - C_j^\top \right\} \\
    (\widehat{C} - C)x^*
    \end{bmatrix}.
\end{align*}

Now we shall show that the mapping $D_0\bar{x}(\cdot)$ is linear. To this end, we first compute the directional derivative of $\bar{x}(\xi)$ and $\xi = 0$. This can be accomplished by showing that $\bar{x}(\xi)$ is locally totally differentiable at $\xi = 0$, followed by applying an appropriate form of the implicit function theorem. Define a vector-valued function $H \in \R^{(k+m)}$ by 
\[
H(x, \xi, \gamma) = \begin{pmatrix}
\nabla_xf(x) + C^\top\gamma + \xi_1 \\
\diag(\gamma)(Cx - d - \xi_2)
\end{pmatrix}.
\] 

Under the additional assumptions \ref{} and \ref{}, the solution of $H(x, \xi, \gamma)=0$ satisfies the KKT condition for \ref{eqn:true-parametrized-nlp-linear-constraints}. In other words in our setting, $H(\bar{x}(\xi), \xi, \bar{\gamma}(\xi))=0$ where $\bar{\gamma}(\xi)$ is the corresponding multipliers. Now by the classical implicit function theorem \citep[e.g.,][Theorem 1B.1]{dontchev2009implicit}, the total derivative at $\xi=0$ can be computed by
\[
\nabla_\xi \bar{x}(0) = - \begin{matrix}
\bm{J}_{x,\gamma} H(\bar{x}(0), 0, \bar{\gamma}(0))
\end{matrix}^{-1}
\begin{bmatrix}
\bm{J}_{\xi} H(\bar{x}(0), 0, \bar{\gamma}(0))
\end{bmatrix},
\]
where in our case,
\[
\bm{J}_{x,\gamma} H(\bar{x}(0), 0, \bar{\gamma}(0)) = \begin{bmatrix}
        \nabla^2_xf(x^*) & C^\top \\
        \diag(\gamma)C & \diag(Cx^*-d) 
        \end{bmatrix},
\]
and
\[
\bm{J}_{\xi} H(\bar{x}(0), 0, \bar{\gamma}(0)) = \begin{bmatrix}
        \bm{1} \\
        \diag(\gamma)\bm{1}
        \end{bmatrix}.
\]
Here the inverse of $\begin{matrix}
\bm{J}_{x,\gamma} H(\bar{x}(0), 0, \bar{\gamma}(0))
\end{matrix}$ always exists. Therefore we finally obtain that
\begin{align*}
    D_0\bar{x}(n^{1/2}\zeta) \xrightarrow{d} \begin{bmatrix}
        \nabla^2_xf(x^*) & C^\top \\
        \diag(\gamma)C & \diag(Cx^*-d) 
        \end{bmatrix}^{-1} \begin{bmatrix}
        \bm{1} \\
        \diag(\gamma)\bm{1}
        \end{bmatrix} \Upsilon,
\end{align*}
which, by Slutsky's theorem, implies 
\begin{align*}
    n^{1/2}\left(\widehat{x} - x^* \right) \xrightarrow{d} .
\end{align*}


\end{proof}
